# Supplementary material for: MultiHiertt: Numerical Reasoning over Multi Hierarchical Tabular and Textual Data
Source: arXiv:2206.01347 source file (2022-06-03)
Supplement: Supplementary file 1 [file interface.tex]

\section{More Details on Dataset}
\subsection{Data Filtering}
\label{data_filtering}
We use following constraints to filter documents:
\begin{itemize}
    \item 
\end{itemize}
